# Supplementary material for: Analyzing Visual Representations in Embodied Navigation Tasks
Source: arXiv:2003.05993 source file (2020-03-12)
Supplement: Supplementary file 1 [file supplement_main.tex]

\documentclass{article}

    \PassOptionsToPackage{numbers, sort&compress}{natbib}

\usepackage{neurips}

\usepackage[utf8]{inputenc} %
\usepackage[T1]{fontenc}    %
\usepackage{url}            %
\usepackage{booktabs}       %
\usepackage{amsfonts}       %
\usepackage{nicefrac}       %
\usepackage{microtype}      %

\usepackage{comment}
\usepackage{caption}
\usepackage{subcaption}
\usepackage{inconsolata}
\usepackage{paralist}
\usepackage{url}
\usepackage{xspace}
\usepackage{amssymb}
\usepackage{times}
\usepackage{epsfig}
\usepackage{graphicx}
\usepackage{amsmath}

\usepackage{algorithm}
\usepackage{algpseudocode}

\usepackage{multirow}
\usepackage{rotating}
\usepackage{booktabs}

\usepackage{enumitem}
\usepackage{paralist}

\usepackage{soul}
\setstcolor{red}

\usepackage[pagebackref=true,breaklinks=true,colorlinks,bookmarks=false,citecolor=green]{hyperref}

\usepackage{amsmath,amsfonts,bm}

\def\eqref#1{equation~\ref{#1}}

\def\1{\bm{1}}

\DeclareMathAlphabet{\mathsfit}{\encodingdefault}{\sfdefault}{m}{sl}
\SetMathAlphabet{\mathsfit}{bold}{\encodingdefault}{\sfdefault}{bx}{n}

\input{space_saver.tex}
\input{definitions.tex}

\title{Insights on Visual Representations \\for Embodied Navigation Tasks \\Supplementary Material}

\author{%
  David S.~Hippocampus\thanks{Use footnote for providing further information
    about author (webpage, alternative address)---\emph{not} for acknowledging
    funding agencies.} \\
  Department of Computer Science\\
  Cranberry-Lemon University\\
  Pittsburgh, PA 15213 \\
  \texttt{hippo@cs.cranberry-lemon.edu} \\
}

\begin{document}

\maketitle

\input{sections/supplement/supplement_content.tex}

\clearpage
{
\bibliography{strings,main}
\bibliographystyle{ieeetr}
}

\end{document}
